# Supplementary material for: On Relaxed Locally Decodable Codes for Hamming and Insertion-Deletion Errors
Source: arXiv:2209.08688 source file (2022-09-19)
Supplement: Supplementary file 1 [file appendix.tex]

\section{On the deterministic output of the decoder} \label{sec:appendix}

In \cref{sec:2qrldc}, we assumed the relaxed decoder $\Dec(i,\cdot)$ for a 2-query weak RLDC has deterministic output conditioned on the queries $j, k$. Here we explain the reason behind this assumption.

Given an index $i \in [n]$ and queries $j,k$ made by $\Dec(i,\cdot)$, in the most general setting the output could be a random variable which depends on $i$ and $y_j$, $y_k$, where $y_j$, $y_k$ are the answers to queries $j$, $k$, respectively. An equivalent view is that the decoder picks a random function $f$ according to some distribution $D_{j,k}^{i}$, and outputs $f(y_j, y_k)$. Here $D_{j,k}^{i}$ is a distribution over all functions $\{f \colon \set{0,1}^2 \rightarrow \set{0,1,\perp} \}$.

We claim that one can use a single \emph{deterministic} function $f_D\colon \set{0,1}^2 \rightarrow \set{0,1,\perp}$ in place of the random function $f \sim D_{j,k}^{i}$, while preserving perfect completeness and the relax decoding property (for the same parameters). We say a pair $(a,b) \in \zo^2$ is achievable if there exists $x \in \zo^n$ such that $(C(x)_j, C(x)_k)=(a,b)$. Otherwise we say $(a,b)$ is unachievable. A simple consequence of the perfect completeness property is that, any two functions $f_1, f_2$ in the support of $D_{j,k}^{i}$ must agree on achievable pairs. Furthermore, the value they agree on cannot be $\perp$. Therefore, we can define $f_D$ as follows:
\begin{align*}
    \forall (a, b) \in \zo^2, \quad f_D(a,b) = \begin{cases}
    0 & \textup{if $f(a,b)=0$ for all $f \in \textup{supp}(D_{j,k}^{i})$} \\
    1 & \textup{if $f(a,b)=1$ for all $f \in \textup{supp}(D_{j,k}^{i})$} \\
    \perp & \textup{otherwise}
    \end{cases}.
\end{align*}
It is easily verified that $f_D$ satisfies perfect completeness. Indeed, whenever the output is $\perp$, it entails the decoder read an unachievable pair, which can only occur in a corrupted codeword. Also note that for any function $f \in \textup{supp}(D_{j,k}^{i})$, either $f_D$ agrees with $f$ on $(a,b)$, or $f_D(a,b)=\perp$. Therefore, $f(a,b) \in \set{x_i, \perp}$ implies $f_D(a,b) \in \set{x_i, \perp}$, and the relaxed decoding property is preserved.

%\jeremiah{One technicality which should be easy to address. What if $\Dec(i, \cdot)$ randomly selects $(j,k)$ and then randomly selects the function $f_{j,k}^i$ from some distribution. By perfect correctness if there are two functions $f_{j,k}^i$ and ${f_{j,k}^{i}}'$ in the support then they need to agree i.e., for any $b_1,b_2 \in \{0,1\}$ either $f_{j,k}^i(b_1,b_2) = {f_{j,k}^{i}}'(b_1,b_2)$ or one of the functions outputs $\bot$ on input $b_1,b_2$. As long as there exists some $f_{j,k}^i$ in the support with $\ell$ bots in the truth table we can add $\{j,k\}$ to $F_{i}^{(\ell)}$} 
